# Supplementary material for: Compression of GPS Trajectories using Autoencoders
Source: arXiv:2301.07420 source file (2023-01-18)
Supplement: Supplementary file 1 [file appendix.tex]

% -------------------------------------------------------------------------------------------------
%      MDSG Latex Framework
%      ============================================================================================
%      File:                  appendix.tex
%      Author(s):             Michael Duerr
%      Version:               1
%      Creation Date:         30. Mai 2010
%      Creation Date:         30. Mai 2010
%
%      Notes:                 - Place your appendix here
%                             - Use the same commands (`chapter', `section', ...) as in main text
% -------------------------------------------------------------------------------------------------
%
\chapter{Examples for Trajectory Length 20}\label{appendix:length_20}
In this appendix, a randomly chosen trajectory (solid black line with square
vertices) is shown with its interpolated TD-TR compression and autoencoder
reconstruction respectively (dashed grey line with cross vertices). The
compression ratios 2, 4, and $6\frac{2}{3}$ are shown.

\begin{figure}[hpbt]
	\centering
	\subfloat[Interpolated TD-TR compression]{
		\includegraphics[width=.9\textwidth]{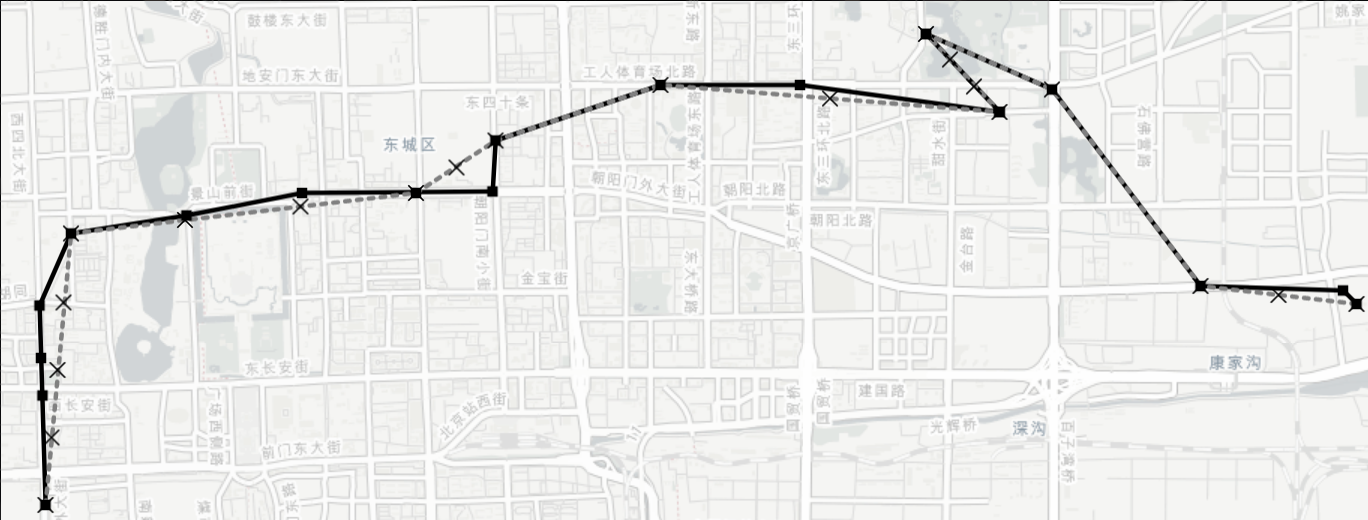}
	}\\
	\subfloat[Autoencoder Reconstruction]{
		\includegraphics[width=.9\textwidth]{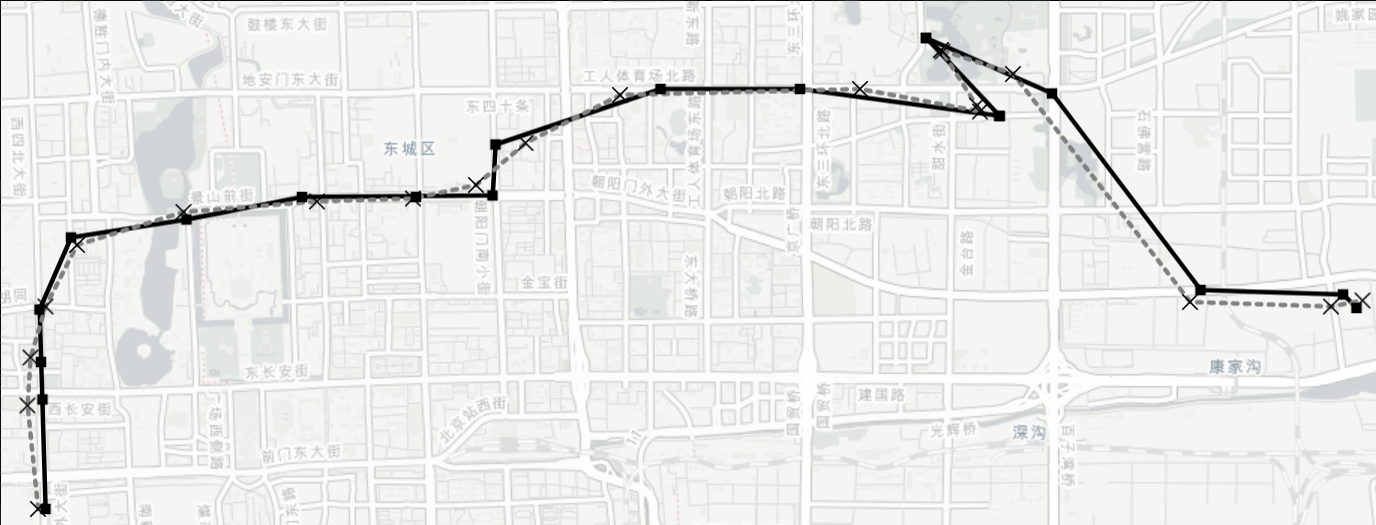}
	}
	\caption{Example trajectory with compressions/reconstructions. CR: 2,
	length: 20.}
\end{figure}

\begin{figure}[hpbt]
	\centering
	\subfloat[Interpolated TD-TR compression]{
		\includegraphics[width=.9\textwidth]{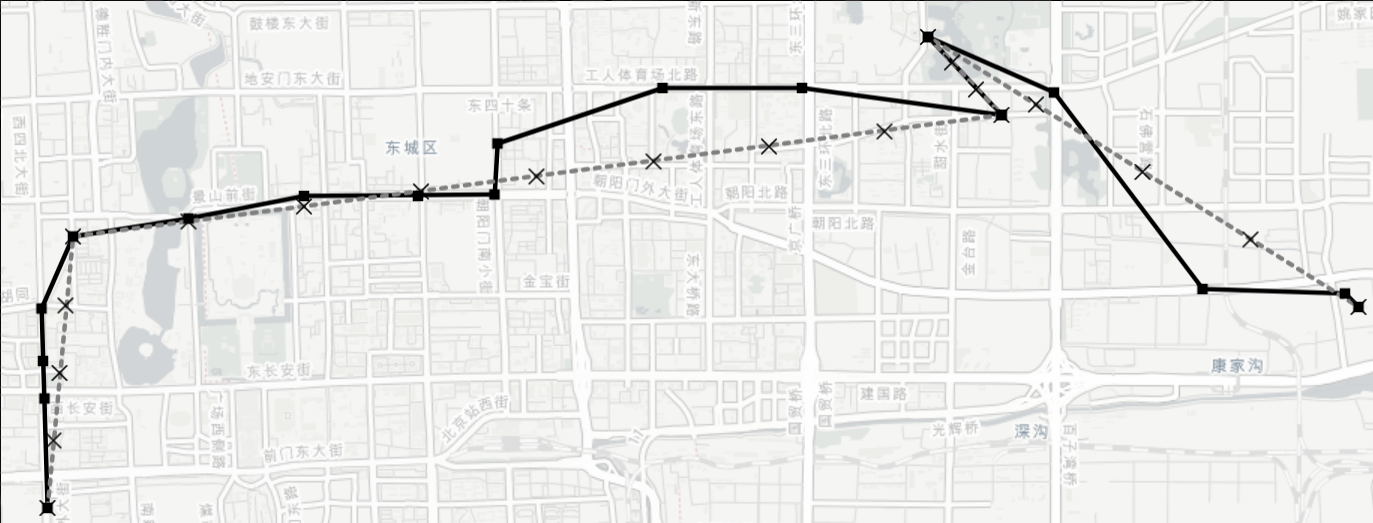}
	}\\
	\subfloat[Autoencoder Reconstruction]{
		\includegraphics[width=.9\textwidth]{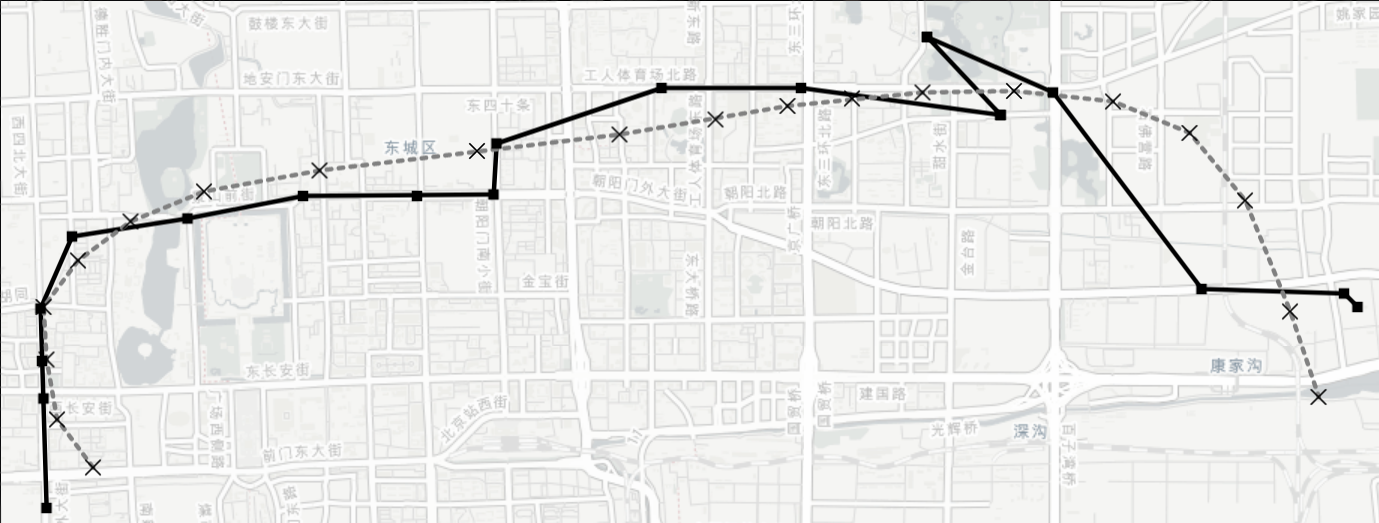}
	}
	\caption{Example trajectory with compressions/reconstructions. CR: 4,
	length: 20.}
\end{figure}

\begin{figure}[hpbt]
	\centering
	\subfloat[Interpolated TD-TR compression]{
		\includegraphics[width=.9\textwidth]{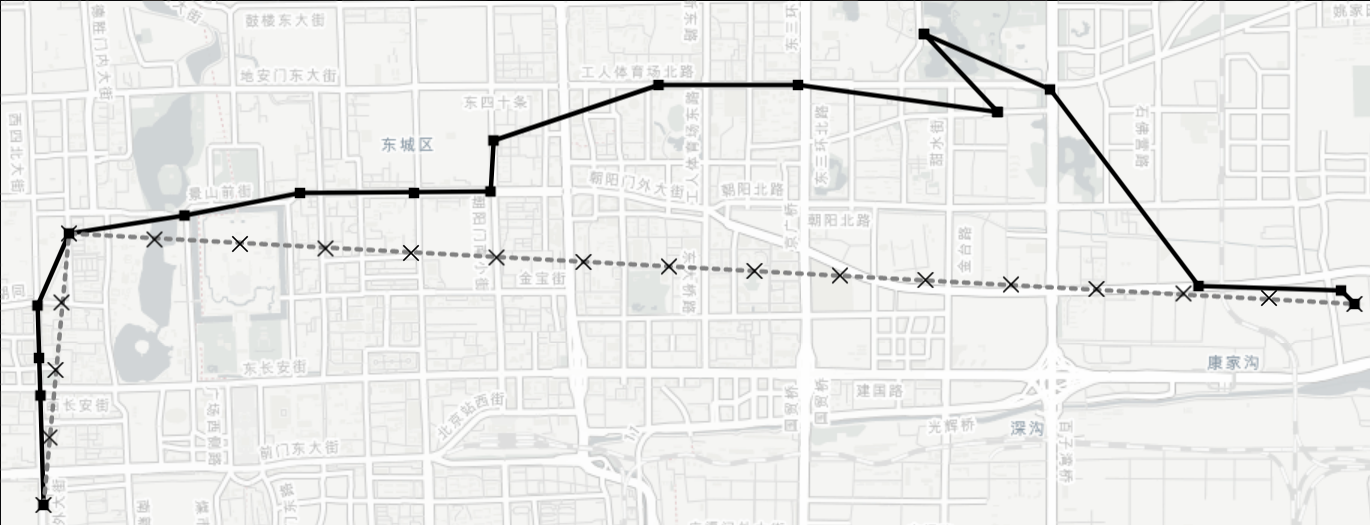}
	}\\
	\subfloat[Autoencoder Reconstruction]{
		\includegraphics[width=.9\textwidth]{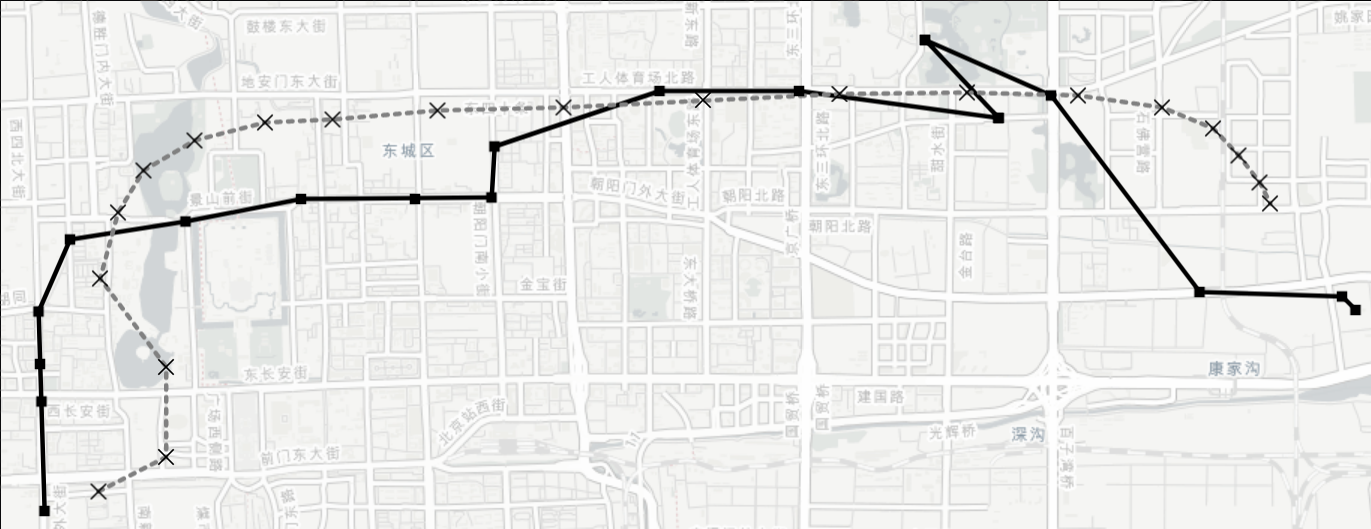}
	}
	\caption{Example trajectory with compressions/reconstructions. CR:
	6$\frac{2}{3}$, length: 20.}
\end{figure}

\chapter{Examples for Trajectory Length 40}\label{appendix:length_40}
In this appendix, a randomly chosen trajectory (solid black line with square
vertices) is shown with its interpolated TD-TR compression and autoencoder
reconstruction respectively (dashed grey line with cross vertices). The
compression ratios 2, 4, 8 and 10 are shown.

\begin{figure}[hpbt]
	\centering
	\subfloat[Interpolated TD-TR compression]{
		\includegraphics[width=.48\textwidth]{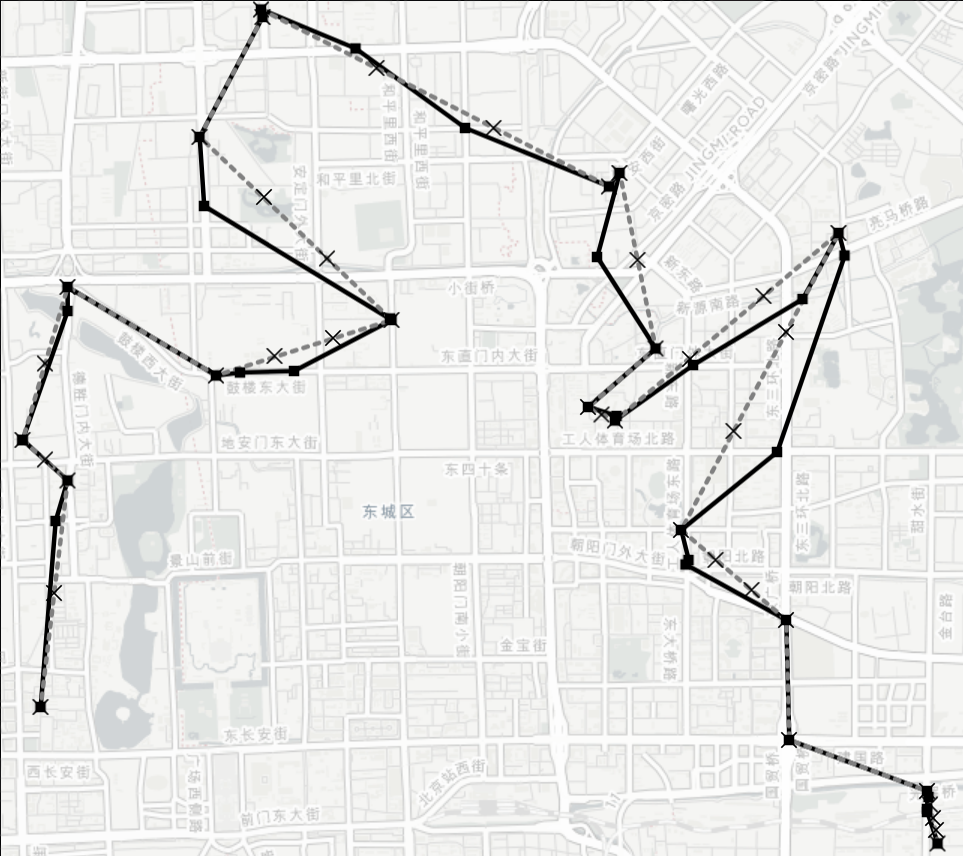}
	}
	\subfloat[Autoencoder Reconstruction]{
		\includegraphics[width=.48\textwidth]{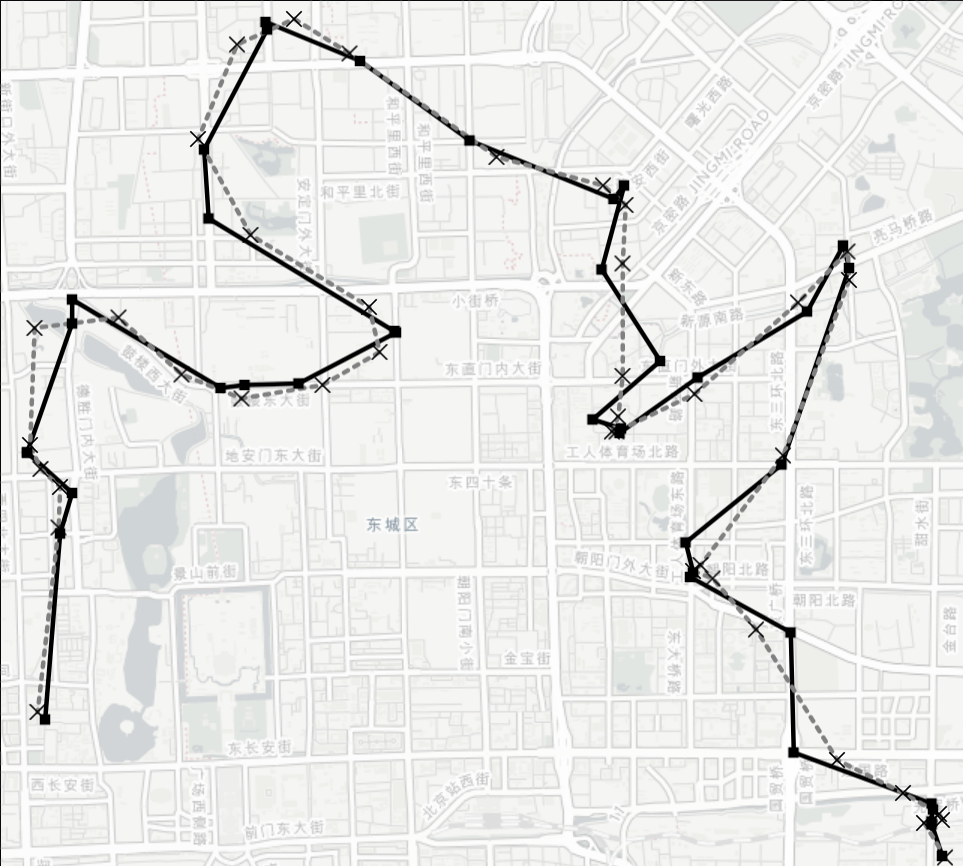}
	}
	\caption{Example trajectory with compressions/reconstructions. CR: 2,
	length: 40.}
\end{figure}

\begin{figure}[hpbt]
	\centering
	\subfloat[Interpolated TD-TR compression]{
		\includegraphics[width=.48\textwidth]{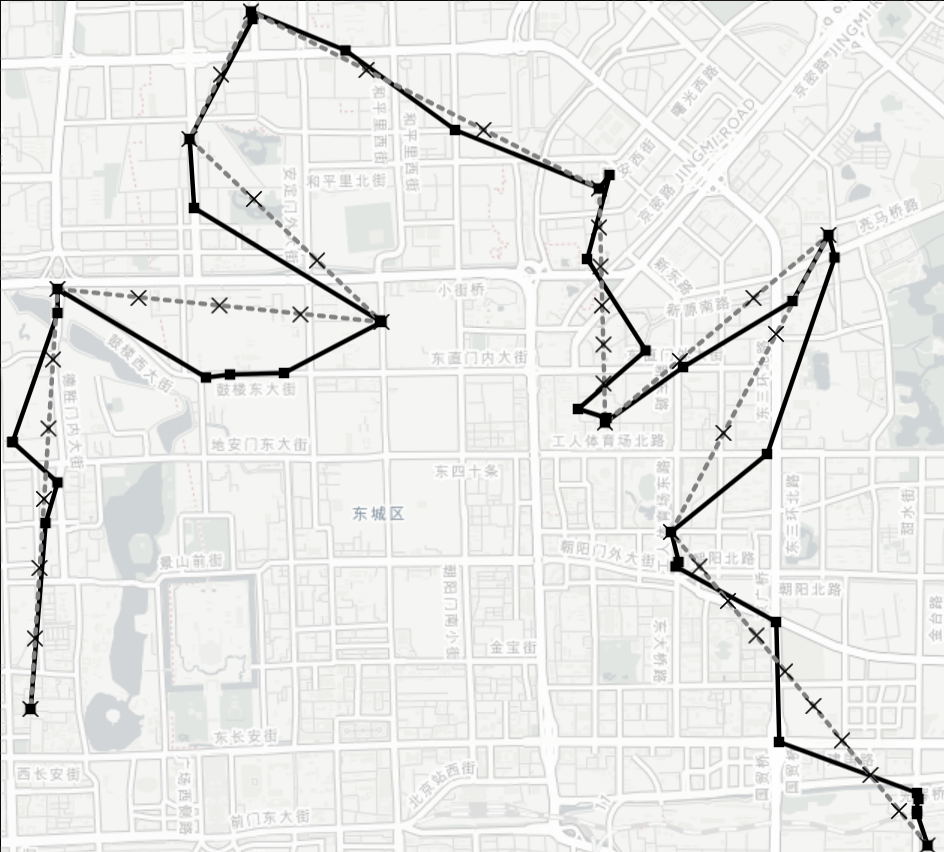}
	}
	\subfloat[Autoencoder Reconstruction]{
		\includegraphics[width=.48\textwidth]{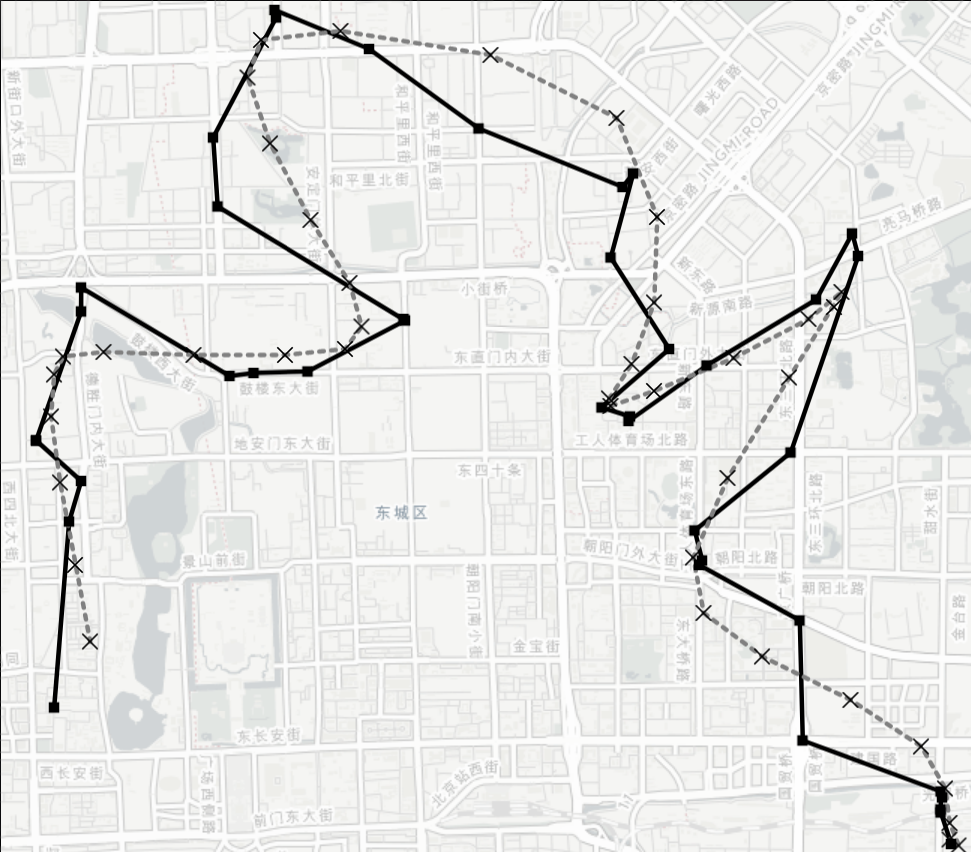}
	}
	\caption{Example trajectory with compressions/reconstructions. CR: 4,
	length: 40.}
\end{figure}

\begin{figure}[hpbt]
	\centering
	\subfloat[Interpolated TD-TR compression]{
		\includegraphics[width=.48\textwidth]{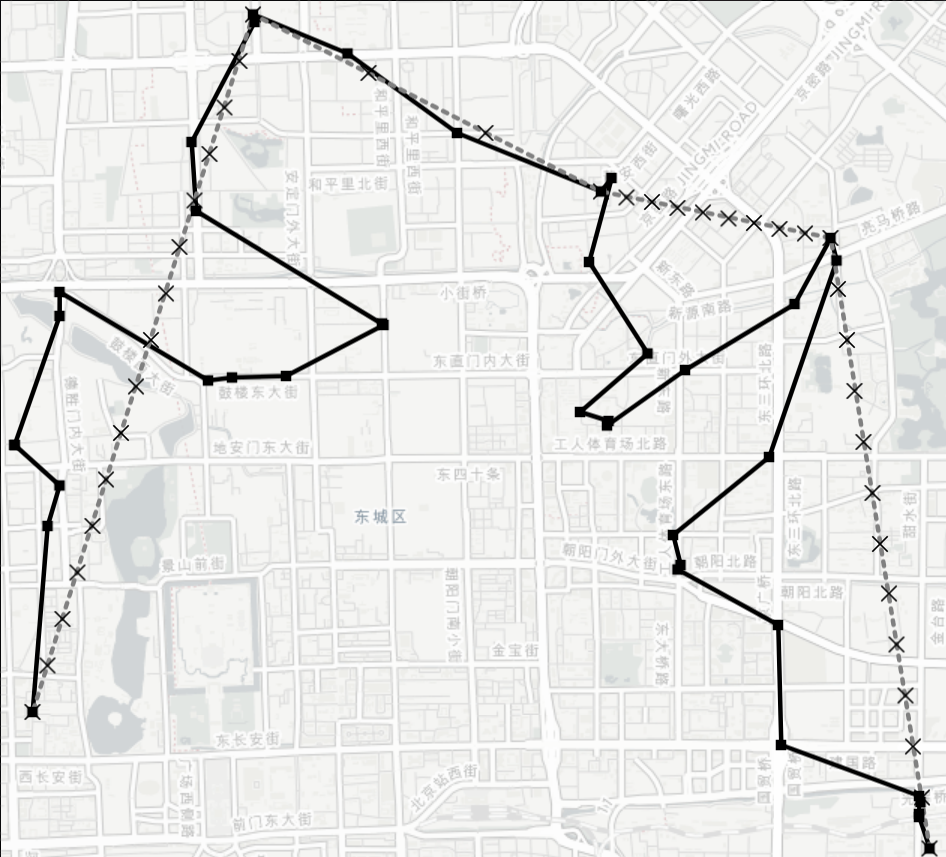}
	}
	\subfloat[Autoencoder Reconstruction]{
		\includegraphics[width=.48\textwidth]{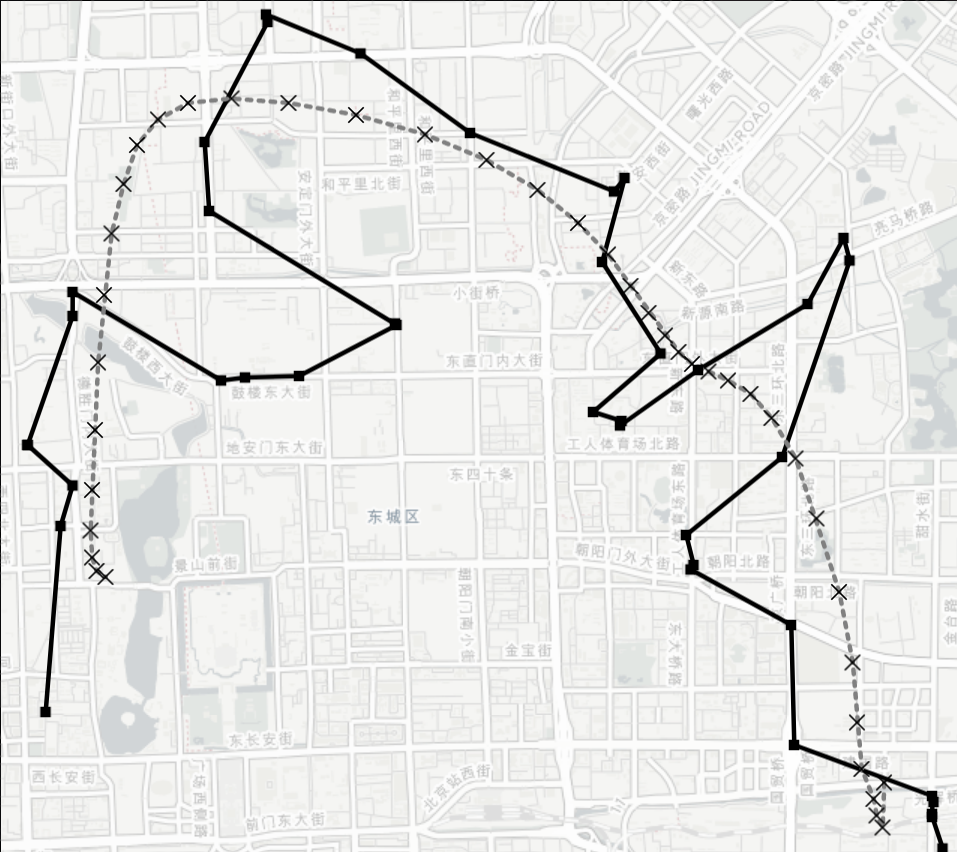}
	}
	\caption{Example trajectory with compressions/reconstructions. CR: 8,
	length: 40.}
\end{figure}

\begin{figure}[hpbt]
	\centering
	\subfloat[Interpolated TD-TR compression]{
		\includegraphics[width=.48\textwidth]{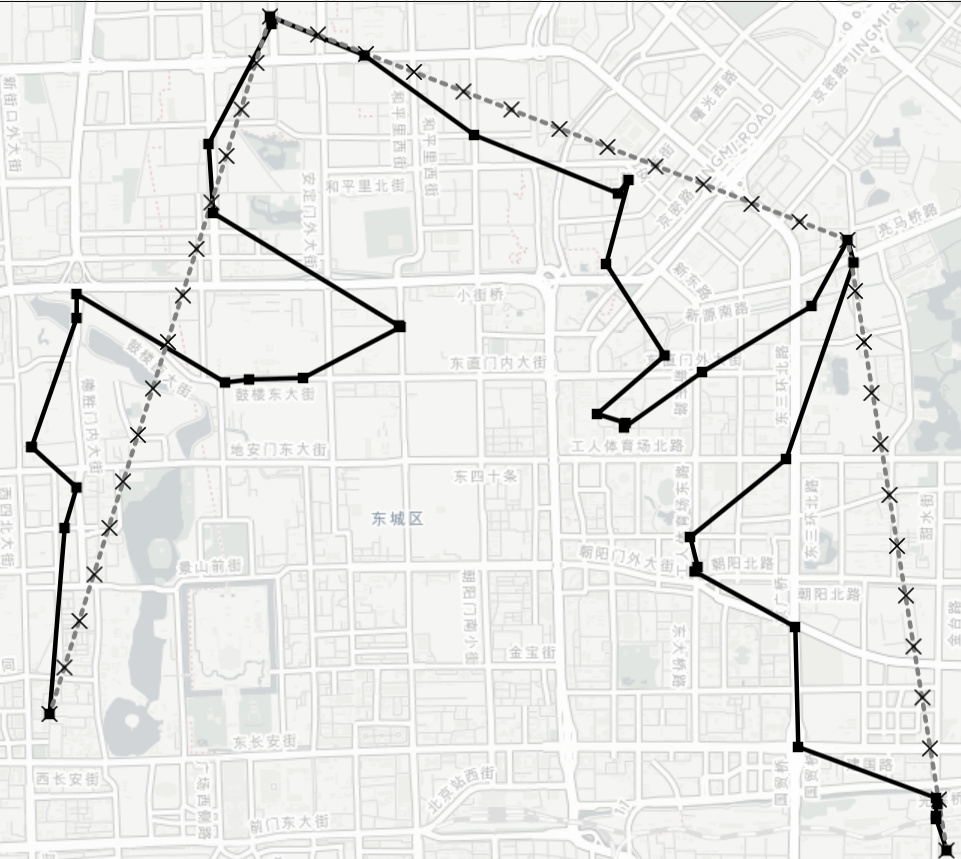}
	}
	\subfloat[Autoencoder Reconstruction]{
		\includegraphics[width=.48\textwidth]{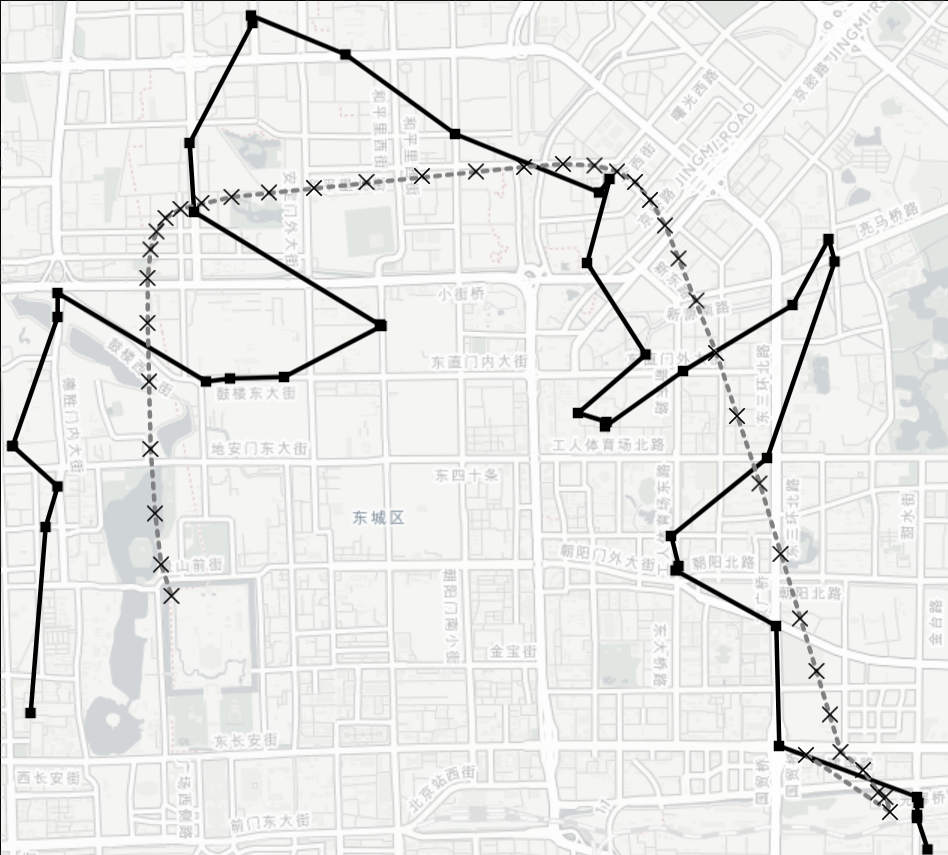}
	}
	\caption{Example trajectory with compressions/reconstructions. CR: 10,
	length: 40.}
\end{figure}
